# Supplementary material for: Drillboards: Adaptive Visualization Dashboards for Dynamic Personalization of Visualization Experiences
Source: arXiv:2410.12744 source file (2025-02-17)
Supplement: Supplementary file 1 [file appendix.tex]

% ----------------------------------------------------------------
%   Appendix: all additional analyses should be here.
% ----------------------------------------------------------------
\appendix

% \section{ScannerDeeply Trained without Pre-processing}
% \label{appendix:trained-on-raw-data}

% that's it!
